# Supplementary material for: Calibration Strategies for Robust Causal Estimation: Theoretical and Empirical Insights on Propensity Score-Based Estimators
Source: arXiv:2503.17290 source file (2025-05-19)
Supplement: Supplementary file 1 [file calibration_classification_appendix.tex]

Early work by \citet{zadrozny2001calibiontrees} demonstrates that decision tree-based models can exhibit high bias as they aim for uniformity in their leaves, which shifts observed frequencies toward extreme values. These models also face high variance when leaves rely on small training samples. Predicting overconfident propensity scores close to 0 or 1 blows up the weights of inverse propensity based estimators leading to unstable treatment effect estimation. This holds especially true for boosting algorithms \citep{blasiok2023doesoptimizingproperloss}. Bagging or random forest that average predictions from a base set of learners struggle to predict values near 0 and 1, due to variance in the underlying base learners \citep{niculescu2005calibclassifier}. \citet{blasiok2023doesoptimizingproperloss} show that logistic regression, which is often considered well-calibrated \citep{niculescu2005calibclassifier, johansson2023wellcalibrated, pedregosa2018scikitlearnmachinelearningpython}, can also be affected by poor calibration through the linear form restriction. \citet{bai2021dontjustblameoverparametrization} show that even when logistic regression is correctly specified, it remains inherently overconfident, indicating that calibration error is intrinsic to the model. The calibration error decreases as the sample size grows relative to the number of parameters, but the overconfidence effect persists. This highlights that propensity scores are often not well calibrated, such that the estimated treatment probabilities may not be reliable across subgroups. Even though theoretical and simulation-based studies address the topic of poor calibration, it is often not addressed transparently in applied causal analysis.
